# Supplementary material for: Online Learning Demands in Max-min Fairness
Source: arXiv:2012.08648 source file (2020-12-15)
Supplement: Supplementary file 1 [file supplementary.pdf]

## 512 Appendix

### 513 A On Max-min Fairness

514 In this section we state and prove some properties about Max-min fairness (MMF) that will be used  
515 in our proofs. Recall that MMF is outlined in Algorithm 1.

516 **Property 1.** *If agent  $i$  reports  $d_i < e_i$ , her allocation is  $d_i$ .*

517 *Proof.* In Algorithm 1,  $d_j < e_j$  for all agents  $j$  before user  $i$  in the sorted order; therefore,  $r/e$  is  
518 increasing until it reaches agent  $i$ . Since  $r/e = 1$  at the beginning, we have  $r/e \geq 1$  until we check  
519 the **if** condition in line 3 for user  $i$ . As  $d_j/e_j < r/e$  for all agents  $j$  until  $i$ , the for loop does not  
520 break, and  $i$  is allocated  $d_i$  in line 4.  $\square$

521 **Property 2.** *If user  $i$  reports  $d_i \geq e_i$ , her allocation is at least  $e_i$ .*

522 *Proof.* We will first argue by way of induction that in Algorithm 1,  $r \geq e$  each time we visit line 3.  
523 For the first user, this is true since  $r = e = 1$ . Now assume that it is true when the **if** condition is  
524 satisfied for a user  $j$ . Then,  $d_j/e_j < r/e$ . We therefore have,

$$\frac{r - d_j}{e - e_j} > \frac{r - re_j/e}{e - e_j} = \frac{r}{e} \cdot \frac{1 - e_j/e}{1 - e_j/e} \geq 1. \quad (6)$$

525 Therefore, the statement is true when we visit line 3 the next time.

526 Now, in Algorithm 1, if a user was allocated her resource in line 4, then  $a_i = d_i > e_i$ . Therefore, say  
527 she was allocated in line 7. When the condition in line 3 is violated for some user,  $r/e > 1$  by the  
528 above argument in (6). Therefore, for all users  $j$  who are assigned in 7,  $a_j = e_j \frac{r}{e} \geq e_j$ .  $\square$

529 **Property 3.** *Suppose we have a demand vector  $d$  and allocation vector  $a$  returned by MMF, where,  
530 for user  $i$ ,  $a_i < d_i$ . Keeping all other reported demands constant, user  $i$ 's allocation would have  
531 been the same for all of her reports  $d'_i \geq a_i$ .*

532 *Proof.* If  $a_i < d_i$ , then this could have been only because she was allocated at line 7 in Algorithm 1.  
533 Therefore, for any bid greater than or equal to  $a_i$ , while her ranking may have changed, she would still  
534 have been allocated the same amount in line 7, which does not depend on her reported demand.  $\square$

535 **Property 4.** *Fix the reported demands of all agents except  $i$ . Let the utilities of agent  $i$  when reporting  
536  $d_i, d_i^*$  be  $\tilde{u}_i$  and  $\tilde{u}_i^*$  respectively. If  $d_i < d_i^*$ , then  $\tilde{u}_i \leq \tilde{u}_i^*$ .*

537 *Proof.* This follows from monotonicity of the utility and the fact that an agent's allocation cannot  
538 decrease when she increases her bid, when all other bids are unchanged.  $\square$

539 **Property 5.** *Fix the reported demands of all agents except  $i$ . Let the utilities of agent  $i$  when reporting  
540  $d_i, d_i^*$  be  $\tilde{u}_i$  and  $\tilde{u}_i^*$  respectively. If  $d_i > d_i^*$ , then  $\tilde{u}_i = \tilde{u}_i^*$ .*

541 *Proof.* Assume the allocation was  $a^*$  when the user reports  $d_i^*$ . If the agent was allocated  $a_i^* < d_i^*$ ,  
542 this follows by Property 3. Now say the agent was allocated  $a_i^* = d_i^*$ , and it changes to  $a_i$  when she  
543 switches to  $d_i$ . As the allocation by MMF does not decrease when an agent increases her demand,  
544  $a_i \geq a_i^*$ . The claim follows from the fact that  $u_i(a) = u_i(a_i^*)$  for all  $a \geq a_i^*$ .  $\square$

545 The above properties lead to the following theorem which establishes efficiency, fairness, and  
546 strategy-proofness for MMF.

547 **Theorem 5.** *MMF (Algorithm 1) is efficient, fair, and strategy-proof.*

548 **Proof. Efficiency:** Assume all users report truthfully. Recall that a mechanism is efficient if  
549  $\ell(d^*, a) = \min(\ell^{\text{ur}}(a) + \ell^{\text{or}}(d^*, a), \ell^{\text{ud}}(d^*, a)) = 0$  where  $\ell^{\text{ur}}, \ell^{\text{or}}, \ell^{\text{ud}}$  are as defined in (1). Since  
550 MMF never allocates a user more than her reported demand,  $\ell^{\text{or}}(d^*, a) = 0$ . Therefore, if  $\ell^{\text{ur}}(a) = 0$ ,  
551 then  $\ell(d^*, a) = 0$ . If  $\ell^{\text{ur}}(a) > 0$ , this means Algorithm 1 never entered line 7 and therefore  $a_i = d_i^*$   
552 for all users  $i$ . Hence,  $\ell(d^*, a) \leq \ell^{\text{ud}}(d^*, a) = 0$ .

553 **Fairness:** Assume user  $i$  reports truthfully. If  $d_i^* < e_i$ , then by Property 1,  $u_i(e_i) = u_i(d_i^*) = u_i(a_i)$ .  
554 If  $d_i^* \geq e_i$ , then by Property 2 and the fact that  $u_i$  is non-decreasing,  $u_i(e_i) \leq u_i(a_i)$ .

555 **Strategy-proofness:** This follows from Properties 4 and 5.  $\square$

## 556 B Notation & Intermediate Lemmas

557 In this section, we state and prove some intermediate results that will be useful in our proofs of  
558 Theorems 1-4. We begin with some notation.

559 **Instantaneous losses:** Let  $\ell_t = \ell(d_{it}^*, a_t)$  be the loss at round  $t$  and  $\ell_t^{\text{ur}} = \ell^{\text{ur}}(a_t)$ ,  $\ell_t^{\text{or}} = \ell^{\text{or}}(d_{it}^*, a_t)$ ,  
560 and  $\ell_t^{\text{ud}} = \ell^{\text{ud}}(d_{it}^*, a_t)$  be the unallocated resources, over allocated resources, and unmet demand  
561 respectively at round  $t$  (1). Recall,  $\ell_t = \min(\ell_t^{\text{ur}} + \ell_t^{\text{or}}, \ell_t^{\text{ud}})$ .

562 **Upper/lower (confidence) bounds on the demands:** Throughout our proofs,  $\hat{\eta}_{it}$  and  $\check{\eta}_{it}$  will denote  
563 upper and lower (confidence) bounds on agent  $i$ 's unit demands  $\eta_i^*$  at round  $t$ ; they satisfy  $\check{\eta}_{it} \leq$   
564  $\eta_i^* \leq \hat{\eta}_{it}$ . Moreover, unless otherwise specified,  $\hat{d}_{it} = w_{it}\hat{\eta}_{it}$  and  $\check{d}_{it} = w_{it}\check{\eta}_{it}$  will denote upper and  
565 lower (confidence) bounds on agent  $i$ 's demand  $d_{it}^*$  for round  $t$ .

566 **Exploration phase & bracket indices in Algorithm 2:** We will use  $\mathbf{E}$  to denote the round indices  
567 belonging to the exploration phase, in Algorithm 2. We will use  $q_t$  to denote the bracket index round  
568  $t$  belongs to and  $T_q$  to denote the number of rounds completed by  $q$  brackets. Then,

$$T_{q_t-1} < t \leq T_{q_t}. \quad (7)$$

### 569 Bounds on the Loss and Fairness

570 The following lemma will be useful in bounding the loss in round  $t$  for Algorithm 2.

571 **Lemma 6.** Suppose on round  $t$ , a multi-round mechanism chose its allocations via MMF by using  
572 an upper bound  $\hat{d}_{it}$  for  $d_{it}^*$  for all  $i \in \{1, \dots, n\}$  as the reported demand. Moreover, let  $\check{d}_{it}$  be a  
573 lower bound for  $d_{it}^*$  for all  $i$ . Then,  $\ell_t \leq \sum_{i=1}^n (\hat{d}_{it} - \check{d}_{it})$ .

574 **Proof.** First, let  $\ell_t^{\text{ur}} > 0$ . This means, in Algorithm 1, all agents were allocated in line 4 and therefore  
575  $a_{it} = \hat{d}_{it} > d_{it}^*$  for all  $i$ . Hence  $\ell_t \leq \ell_t^{\text{ud}} = 0$ . The statement is true since  $\hat{d}_{it} \geq \check{d}_{it}$ .

576 Now let  $\ell_t^{\text{ur}} = 0$ . We bound  $\ell_t \leq \ell_t^{\text{or}} = \sum_i \max(a_{it} - d_{it}^*)$ . Since the mechanism reports  $\hat{d}_{it} = w_{it}\hat{\eta}_{it}$   
577 as the demand to MMF, and since MMF does not allocate more than the reported demand, we have  
578  $a_{it} \leq \hat{d}_{it}$ . The claim follows since  $d_{it}^* \geq \check{d}_{it}$ .  $\square$

579 The following lemma will be useful in the proofs of our fairness results.

580 **Lemma 7.** Suppose on round  $t$ , the allocations  $a_t$  are set via MMF, and that for agent  $i$  we used  
581 a reported demand  $d_{it} = \eta_{it}w_{it}$ . Let  $\hat{\eta}_{it}$  be an upper bound on  $\eta_i^*$  which further satisfies  $\hat{\eta}_{it} \geq \eta_{it}$ .  
582 Then, regardless of the behaviour of the other agents, we have for agent  $i$ ,

$$u_i(e_i/w_{it}) - u_i(a_{it}/w_{it}) \leq L_i(\hat{\eta}_{it} - \eta_{it}).$$

583 **Proof.** Denote  $\hat{d}_{it} = \hat{\eta}_{it}w_{it}$  and  $d_{it}^* = \eta_i^*w_{it}$ . First observe that if  $d_{it} > e_i$ , by Property 2, we have  
584  $u_i(e_i/w_{it}) - u_i(a_{it}/w_{it}) \leq 0$  and the statement is true since the RHS is positive. Now say  $d_{it} < e_i$ .  
585 By Property 1,  $a_{it} = d_{it}$  and therefore,

$$\begin{aligned} u_i(e_i/w_{it}) - u_i(d_{it}/w_{it}) &\leq u_i(e_i/w_{it}) - u_i(d_{it}^*/w_{it}) + u_i(d_{it}^*/w_{it}) - u_i(d_{it}/w_{it}) \\ &\leq L_i(d_{it}^*/w_{it} - d_{it}/w_{it})^+ \leq L_i(\hat{\eta}_{it} - \eta_{it}). \end{aligned}$$

586 Above, we have used  $u_i(e_i/w_{it}) - u_i(d_{it}^*/w_{it}) \leq 0$  by Theorem 5 and the fact that  $u_i$  is  $L_i$  Lipschitz  
 587 and increasing. The last step uses  $\hat{\eta}_{it} > \eta_i^*$ .  $\square$

## 588 Strategy-proofness

589 We next present some results that will be useful in establishing strategy-proofness for Algorithm 2.  
 590 For this, consider any agent  $i$  and fix the behaviour of all other agents. Let  $U_{iT}, U_{iT}^\pi$  respectively  
 591 denote the sum of utilities when  $i$  participates truthfully and when she is following any other (non-  
 592 truthful) policy  $\pi$ . Let  $\{a_{it}^\pi\}_t, \{a_{it}\}_t$  respectively denote the sequence of allocations for agent  $i$  when  
 593 she is adopting these strategies. Let  $\{\tilde{a}_{it}\}_t$  denote the allocations when agent  $i$  follows  $\pi$  from rounds  
 594 1 to  $t - 1$ , but her allocation for round  $t$  is based on her true unit demand; in Algorithm 2, this means  
 595 we use  $\hat{\eta}_i = \eta_i^*$  in line 5. Note that in general,  $\tilde{a}_{it}$  depends on previous allocations when following  $\pi$ ,  
 596 since it will have also affected the allocations and consequently the estimates of the unit demands  
 597 for the other agents, which in turn will affect the allocation  $\tilde{a}_{it}$  chosen by MMF at round  $t$  for agent  
 598  $i$ . Finally, let  $\{a_{it}^*\}_t$  denote the sequence of allocations for  $i$  when we use the true demands for *all*  
 599 agents.

600 Our next Lemma shows that Algorithm 2 is strategy-proof if our upper bounds are correct.

601 **Lemma 8.** *Algorithm 2 is strategy-proof if  $\hat{\eta}_i$  in line 5 is an upper bound on  $\eta_i^*$ .*

602 *Proof.* We first decompose  $U_{iT}^\pi - U_{iT}$  as follows,

$$\begin{aligned} U_{iT}^\pi - U_{iT} &= \sum_{t=1}^T (u_i(a_{it}^\pi/w_{it}) - u_i(a_{it}^\pi/w_{it})) = \sum_{t \notin \mathbf{E}} (u_i(a_{it}^\pi/w_{it}) - u_i(a_{it}/w_{it})) \\ &\leq \sum_{t \notin \mathbf{E}} (u_i(\tilde{a}_{it}/w_{it}) - u_i(a_{it}/w_{it})) \end{aligned}$$

603 Here, in the second step we have used the fact that when  $t \in \mathbf{E}$ , the allocations are chosen independent  
 604 of the agent's past reports. In the third step we use the fact that MMF is strategy-proof (Theorem 5),  
 605 so the agent's utility is always maximised by using her true demand. We now argue that each term  
 606 in the last sum is 0. This is because the mechanism only uses values in the exploration phase to  
 607 determine allocations, and moreover the allocations in the exploration phase for agent  $j \neq i$  are  
 608 chosen independent of the reports by the agent  $i$ —for the deterministic feedback model,  $j$ 's allocations  
 609 in the exploration phase depend only on its previous reports, and in the stochastic model, they are  
 610 always set to be the entitlements. Therefore, the value used for  $\hat{\eta}_j$  in line (5) is the same for all agents  
 611  $j \neq i$  when computing  $\tilde{a}_{it}$  and  $a_{it}$ . By Property 5, we have  $u_i(\tilde{a}_{it}/w_{it}) - u_i(a_{it}/w_{it}) = 0$ .  $\square$

## 612 Bounding the number of Exploration Phases in Algorithm 2

613 The following two lemmas will help us lower and upper bound the number of brackets  $q_T$  after  $T$   
 614 rounds for the two different models (7).

615 **Lemma 9.** *Suppose we execute Algorithm 2 with  $2n$  exploration phase rounds in each bracket  
 616 followed by  $r'(q) = \lfloor e^q \rfloor$  rounds for the latter phase. Then,*

$$\log \left( \frac{T}{2n + e} \right) \leq q_T \leq 1 + \log(T).$$

617 *Proof.* For brevity, write  $q = q_T$ . Using the notation in (7), we first observe  $T_{q-1} < T \leq T_q$ , where  
 618  $T_m = 2nq + \sum_{t=1}^m \lfloor e^t \rfloor$ . Letting  $S_m = \sum_{t=1}^m e^t$  and bounding the sum of an increasing function by  
 619 an integral we have,

$$\int_0^m e^t dt < S_m < \int_1^{m+1} e^t dt \implies (e^m - 1) < S_m < e(e^m - 1).$$

620 This leads to the following bounds on  $T$ ,

$$T \leq T_q \leq 2nq + \sum_{t=1}^q e^t \leq 2nq + e(e^q - 1) \leq (2n + e)e^q,$$

$$T \geq T_{q-1} \geq 2n(q-1) + \sum_{t=1}^{q-1} (e^t - 1) \geq (2n-1)(q-1) + e^{q-1} - 1 \geq e^{q-1}.$$

621 In the last step, we have used the fact that  $(q-1)(2n-1) - 1 \geq 0$  when  $q \geq 2$  which is true when  
 622  $T \geq 2n+3$ . Inverting the above inequalities yields the claim. For  $T \leq 2n+2$ , the statement can be  
 623 verified easily since  $q_T = 1$ .  $\square$

624 **Lemma 10.** *Suppose we execute Algorithm 2 with 1 exploration phase round in each bracket followed  
 625 by  $r'(q) = \lfloor 5q/6 \rfloor$  rounds for the latter phase. Then,  $\frac{1}{2}T^{2/3} \leq q_T \leq 3T^{2/3}$ .*

626 *Proof.* The claim can be easily verified for  $T = 1$  so let  $T \geq 2$ . The proof will follow along  
 627 similar lines to the proof of Lemma 9. For brevity, write  $q = q_T$ ,  $c = 5/6$ ,  $d = 1/2$ . We have,  
 628  $T_{q-1} < T \leq T_q$ , where,  $T_m = q + \sum_{t=1}^m \lfloor ct^d \rfloor$ . Letting  $S_m = \sum_{t=1}^m t^d$  and bounding the sum of an  
 629 increasing function by an integral we have,

$$\int_0^m t^d dt < S_m < \int_1^{m+1} t^d dt \implies \frac{m^{d+1}}{d+1} < S_m < \frac{(m+1)^{d+1} - 1}{d+1}. \quad (8)$$

630 This leads to the following bounds on  $T$ ,

$$T \leq T_q \leq q + c \sum_{t=1}^q t^d \leq q + \frac{c}{d+1} ((q+1)^{d+1} - 1) \leq q^{d+1} + \frac{c}{d+1} (2q)^{d+1} \leq c_1 q^{3/2}, \quad (9)$$

$$T \geq T_{q-1} \geq (q-1) + \sum_{t=1}^{q-1} (ct^d - 1) \geq \frac{c}{d+1} (q-1)^{d+1} \geq \frac{c}{d+1} \left(\frac{q}{2}\right)^{d+1} = c_2 q^{3/2}. \quad (10)$$

631 Here  $c_1 = 1 + 2^{5/2}c/3$  and  $c_2 = c/(3\sqrt{2})$ . In (9), we have used the upper bound in (8) with  $m = q$ ,  
 632 and the facts  $q \leq q^{3/2}$ ,  $q+1 \leq 2q$ . In (10), we have used the lower bound in (8) with  $m = q-1$ ,  
 633 and that  $q-1 \geq q/2$  when  $q \geq 2$  which is true when  $T \geq 2$ . We therefore have,  $q \leq c_2^{-2/3} T^{2/3}$  and  
 634  $q \geq c_1^{-2/3} T^{2/3}$ . Substituting  $c = 7/8$  yields the desired result.  $\square$

## 635 Technical Lemmas

636 Finally, we will also use the following results in our proofs.

637 **Lemma 11** (de la Pena et al. [19], Corollary 2.2). *Let  $A, B$  be random variables such that  $A > 0$  a.s.  
 638 and  $\mathbb{E} \left[ e^{\gamma B} - \frac{\gamma^2 A}{2} \right] \leq 1$  for all  $\gamma \in \mathbb{R}$ . Then, for all  $c \geq 2$ ,  $\mathbb{P} \left( |B| > cA\sqrt{2 + \log(2)} \right) \leq e^{-c^2/2}$ .*

639 **Lemma 12.** *Let  $c > 0$ . Then, for all  $x \in [0, c]$ ,  $x \leq \frac{c}{\log(1+c)} \log(1+x)$ .*

640 *Proof.* Write  $f(x) = \frac{c}{\log(1+c)} \log(1+x) - x$ . The claim follows by observing that  $f$  is concave and  
 641 that  $f(0) = f(c) = 0$ .  $\square$

## 642 C Proofs of Results in Section 3.1

643 In this section, we present our analysis for the deterministic feedback model.

### 644 C.1 Proof of Theorem 1

645 **Efficiency:** We will first decompose the  $T$ -period loss as follows,

$$L_T \leq \sum_{t \in \mathbf{E}} \ell_t + \sum_{t \notin \mathbf{E}} \ell_t \leq 2nq_T + \sum_{t \notin \mathbf{E}} \ell_t \leq 2n \log(eT) + \sum_{t \notin \mathbf{E}} \sum_{i=1}^n (\hat{d}_{it} - \check{d}_{it}). \quad (11)$$

646 Above, we have used the fact that in  $T$  rounds there will have been  $2nq_T$  exploration rounds and then  
 647 used Lemma 9 to bound  $q_T$ . To bound the second sum, we have used Lemma 6. Here,  $\hat{d}_{it} = w_{it} \hat{\eta}_{it}$

648 and  $\tilde{d}_{it} = w_{it}\tilde{\eta}_{it}$  are upper and lower bounds on the demands, where  $\hat{\eta}_{it}, \tilde{\eta}_{it}$  are the upper and lower  
 649 bounds on the unit demand, computed at the end of the exploration phase in line 2 as described in  
 650 Section 3.1. Since we throttle the load of the agent being explored at a given exploration round, we  
 651 always halve the width of the current upper and lower bounds. We therefore have, for  $t \notin \mathbf{E}$ ,

$$(\hat{d}_{it} - \tilde{d}_{it}) = w_{it}(\hat{\eta}_{it} - \tilde{\eta}_{it}) \leq \frac{w_{\max}\eta_{\max}}{2^{2q_t-1}} \leq \frac{2w_{\max}\eta_{\max}}{4^{\log(\frac{t}{2n+e})}} \leq \frac{2(2n+e)^{\log(4)}w_{\max}\eta_{\max}}{t^{\log(4)}}.$$

652 The second step observes that in  $t$  rounds, there will have been  $q_t$  brackets and therefore  $2q_t$   
 653 exploration rounds for agent  $i$ . We then use the lower bound in Lemma 9 which is positive when  
 654  $T \geq 2n + 3$ . By summing over all agents and time steps, we have

$$\sum_i \sum_{t=1}^n (\hat{d}_{it} - \tilde{d}_{it}) \leq 2 \cdot 5^{\log(4)} w_{\max} \eta_{\max} \frac{\log(4)}{\log(4) - 1} n^{1+\log(4)} \leq 67 w_{\max} \eta_{\max} n^{2.39}.$$

655 The claim on asymptotic efficiency follows by combining this with (11).

656 **Fairness:** We decompose the sum of utilities into  $t \in \mathbf{E}$  and  $t \notin \mathbf{E}$  and apply Lemma 7 to obtain,

$$\begin{aligned} U_{iT}^{e_i} - U_{iT} &= \sum_{t \in \mathbf{E}} (u_i(e_i/w_{it}) - u_i(a_{it}/w_{it})) + \sum_{t \notin \mathbf{E}} (u_i(e_i/w_{it}) - u_i(a_{it}/w_{it})) \\ &\leq \sum_{t \in \mathbf{E}} (u_i(e_i/w_{it}) - u_i(0)) \leq 2nL_i e_i q_T. \end{aligned}$$

657 Above,  $u_i(e_i/w_{it}) - u_i(a_{it}/w_{it}) \leq 0$  for  $t \notin \mathbf{E}$  by applying Lemma 7 with  $\eta_{it}$  and  $\hat{\eta}_{it}$  both set to the  
 658 value  $\hat{\eta}_i$  in line 5 of Algorithm 2 (which is an upper bound on  $\eta_i^*$ ). The last step uses Lipschitzness  
 659 of agent  $i$ 's utility and that in  $T$  rounds there will have been  $2nq_T$  exploration rounds. The claim  
 660 follows by observing  $e_i < 1$  and by applying the upper bound Lemma 9.

661 **Strategy-proofness:** This follows from Lemma 8 as  $\hat{\eta}_i$  is an upper bound on  $\eta_i^*$ .  $\square$

## 662 C.2 Proof of Theorem 2

663 **Efficiency:** First consider the loss at round  $t$ , where, recall  $\ell_t = \min(\ell_t^{\text{ur}} + \ell_t^{\text{or}}, \ell_t^{\text{ud}})$ . If  $\ell_t^{\text{ur}} > 0$ , we  
 664 will bound  $\ell_t \leq \ell_t^{\text{ud}}$  and if  $\ell_t^{\text{ur}} = 0$ , we will bound  $\ell_t \leq \ell_t^{\text{or}}$ . Intuitively, if the resource is scarce  
 665 we will show that we have not been inefficient by over-allocating to users, and if there are excess  
 666 resources, we will show that we have not under-allocated to anyone. This leads us to,

$$L_T = \sum_{t=1}^T \ell_t \leq 1 + \sum_{t \geq 2, \ell_t^{\text{ur}}=0} \ell_t^{\text{or}} + \sum_{t \geq 2, \ell_t^{\text{ur}}>0} \ell_t^{\text{ud}} \leq 1 + \sum_{t=2}^T \ell_t^{\text{or}} + \sum_{t \geq 2, \ell_t^{\text{ur}}>0} \ell_t^{\text{ud}}. \quad (12)$$

667 Consider the first sum in the RHS. Recall that  $\ell_t^{\text{or}} = \sum_{i=1}^n (a_{it} - d_{it}^*)^+$ . We will bound the first sum  
 668 by bounding  $\sum_{t=2}^T (a_{it} - d_{it}^*)^+$  for user  $i$ . Let  $\nu_{it} = a_{it}/w_{it}$ . Moreover, let  $s_1, s_2, \dots$ , denote the  
 669 round indices after the second round in which,  $a_{it} > d_{it}^*$ . Note that  $\nu_{is_1} - \eta_i^* \leq \frac{1}{2}\eta_{\max}$ . We have,

$$\nu_{is_{r+1}} - \eta_i^* \leq \frac{1}{2} (\hat{\eta}_{is_{r+1}} + \tilde{\eta}_{is_{r+1}}) - \eta_i^* = \frac{1}{2} (\nu_{is_r} - \eta_i^*) \leq \dots \leq \frac{1}{2^r} (\nu_{is_1} - \eta_i^*) \leq \frac{\eta_{\max}}{2^{r+1}}.$$

670 Above, the first step uses the fact that the allocations are chosen by MMF, by setting the demand of  
 671 user  $i$  to be  $\eta_i w_{it} = (\hat{\eta}_{is_{r+1}} + \tilde{\eta}_{is_{r+1}}) w_{it}$  and the fact that MMF does not allocated more than the  
 672 reported demand. The second step uses that since we did not over-allocate between rounds  $s_r$  and  
 673  $s_{r+1}$ , the upper bound  $\hat{\eta}_{is_{r+1}}$  at round  $s_{r+1}$  is the unit allocation  $\nu_{is_r}$  at round  $s_{r+1}$ ; additionally,  
 674  $\tilde{\eta}_{it} \leq \eta_i^*$  for all  $t$ . By repeatedly applying this argument, we arrive at the final bound. We have,

$$\sum_{t=2}^T (a_{it} - d_{it}^*) \leq \sum_{r=1}^{\infty} w_{is_r} (\nu_{is_{r+1}} - \eta_i^*) \leq w_{\max} \sum_{r=1}^{\infty} (\nu_{is_{r+1}} - \eta_i^*) \leq w_{\max} \eta_{\max}.$$

675 By summing over all agents we can bound the first sum in (12) by  $nw_{\max}\eta_{\max}$ . Now let us turn to the  
 676 second summation. Since,  $\ell_t^{\text{ur}} > 0$ , we know that at round  $t$ , all agents were allocated their resource  
 677 in line 4 in MMF, and hence  $a_{it} = d_{it} = \eta_{it} w_{it}$ , where, recall  $\eta_{it} = \frac{1}{2}(\hat{\eta}_{it} + \tilde{\eta}_{it})$ . Therefore,

$$\ell_t^{\text{ud}} = \sum_{i=1}^n (d_{it}^* - a_{it})^+ = \sum_{i=1}^n w_{it} (\eta_i^* - \eta_{it})^+ \leq w_{\max} \frac{1}{2} \sum_{i=1}^n (\hat{\eta}_{it} - \tilde{\eta}_{it}).$$

Letting  $s_1, s_2, \dots$ , denote the round indices where  $\ell_t^{\text{ur}} > 0$ , we have

$$\hat{\eta}_{is_{r+1}} - \check{\eta}_{is_{r+1}} \leq \hat{\eta}_{is_r} - \check{\eta}_{is_r} \leq \frac{1}{2} (\hat{\eta}_{is_r} - \check{\eta}_{is_r}) \leq \dots \leq \frac{\eta_{\max}}{2^{r+1}}. \quad (13)$$

The first step above uses that both  $\hat{\eta}_{it}, \check{\eta}_{it}$  are respectively non-decreasing and non-increasing with  $t$  while the second step uses the fact that since  $a_{is_r} = \eta_{is_r} w_{is_r}$  in round  $s_r$ , the gap between the upper and lower bounds would have halved at the next round. By combining the two previous displays, we can bound the second sum in (12) by  $nw_{\max}\eta_{\max}$ . Therefore,  $L_T \leq 1 + 2nw_{\max}\eta_{\max}$ .

**Fairness:** Observe that  $u_i(e_i/w_{it}) < u_i(a_{it}/w_{it})$  only when  $a_{it} < \min(e_i, d_{it}^*)$ ; if  $a_{it} \geq e_i$ , then the agent's utility will be larger since  $u_i$  is non-decreasing and further,  $u_i(\eta_i^*) = u_i(\eta)$  for all  $\eta \geq \eta_i^*$ . Let  $\nu_{it} = a_{it}/w_{it}$ . Letting  $s_1, s_2, \dots$ , denote the round indices where  $a_{it} < \min(e_i, d_{it}^*)$ , we simplify  $U_{iT}^{e_i} - U_{iT}$  as follows.

$$\begin{aligned} U_{iT}^{e_i} - U_{iT} &= \sum_{t=1}^T \left( u_i \left( \frac{e_i}{w_{it}} \right) - u_i \left( \frac{a_{it}}{w_{it}} \right) \right) \\ &\leq \sum_{t: a_{it} \leq \min(e_i, d_{it}^*)} \left( u_i \left( \frac{e_i}{w_{it}} \right) - u_i \left( \frac{d_{it}^*}{w_{it}} \right) + u_i \left( \frac{d_{it}^*}{w_{it}} \right) - u_i \left( \frac{\eta_{it} w_{it}}{w_{it}} \right) \right) \\ &\leq \sum_{r=1}^{\infty} (u_i(\eta_i^*) - u_i(\eta_{is_r})) \leq L_i \sum_{r=1}^{\infty} (\eta_i^* - \eta_{is_r})^+ \leq \frac{L_i}{2} \sum_{r=1}^{\infty} (\hat{\eta}_{is_r} - \check{\eta}_{is_r}) \leq L_i \eta_{\max}. \end{aligned}$$

Above, the second step adds and subtracts  $u_i(\eta_i^*) = u_i(d_{it}^*/w_{it})$  while also observing  $a_{it} = d_{it} = \eta_{it} w_{it}$  by Property 1. The third step uses Theorem 5. The fourth step uses that  $u_i$  is Lipschitz and increasing. The fifth step simply observes  $\eta_i^* \leq \hat{\eta}_{it}$  and  $\eta_{it} = \frac{1}{2}(\hat{\eta}_{it} + \check{\eta}_{it})$  for all  $t$ . The last step uses a similar argument to (13).  $\square$

**Remark 1.** Our proofs used the fact that  $w_{it} > 0$  when arguing that  $\hat{\eta}_{it} - \check{\eta}_{it}$  is halved at the end of each exploration round in Appendix C.1; more concretely, had an agent experienced no traffic during one of her exploration rounds, this would not have been true. This assumption can be avoided by more careful book-keeping where the mechanism checks if an agent has non-zero traffic and if not, delaying that exploration round to a future round.

## D Proofs of Results in Section 3.2

This section presents our analysis for the stochastic feedback model. In Appendix D.1, we will first show that the confidence intervals in (5) traps the true demands with probability larger than  $1 - \delta$  in all rounds. In Appendices D.2 and D.3, we will establish our results for Algorithms 2 and 3 respectively assuming that this is true.

### D.1 Confidence Intervals for $\eta_i^*$

Recall that  $X_{it}$  is drawn from a  $\sigma_{it}$  sub-Gaussian distribution. Letting  $z_{jt} = X_{it} - \mu(a_{it}\theta_i^*/w_{is})$ , we therefore have for all  $i, t$ ,

$$\text{for all } \lambda > 0, \quad \mathbb{E}[e^{\lambda z_{jt}}] \leq \exp\left(\frac{\lambda^2 \sigma_{it}^2}{2}\right). \quad (14)$$

Throughout our proofs, we will assume that both  $\{w_{it}\}_{t \geq 1}$  and  $\{\sigma_{it}\}_{t \geq 1}$  are fixed sequences. The following lemma shows that the probability that the confidence intervals in (5) do not capture the true parameter and demands is bounded by  $\delta$ .

**Lemma 13.** Assume the feedback model described in Section 3.2 and let  $(\check{\theta}_{it}, \hat{\theta}_{it})$  and  $(\check{\eta}_{it}, \hat{\eta}_{it})$  be as defined in (5). Then, with probability greater than  $1 - \delta$ , for all  $i \in \{1, \dots, n\}$  and all  $t \geq 0$ ,

$$\theta_i^* \in (\check{\theta}_{it}, \hat{\theta}_{it}), \quad \eta_i^* \in (\check{\eta}_{it}, \hat{\eta}_{it}).$$

*Proof.* We will divide this proof into three steps.

710 **Step 1:** Consider any user  $i$ . First, we will show that the sum of deviations of  $X_{it}$  from the true  
 711 payoff scale with  $A_{it}$ . This part of the analysis is based on Rusmevichientong and Tsitsiklis [44].  
 712 Define,

$$B_{it} = \sum_{s=1}^{t-1} \frac{a_{is}}{w_{it}\sigma_{is}^2} z_{is}, \quad \text{where, } z_{is} = X_{is} - f_{\theta_i^*}(a_{is}/w_{is}) = X_{is} - \mu(a_{is}\theta_i^*/w_{is}).$$

713 We will now apply Lemma 11 with  $A \leftarrow A_{it}^2$  and  $B \leftarrow B_{it}$ . We first need to verify that the  
 714 condition for the Lemma holds. Let  $\gamma \in \mathbb{R}$  be given. Writing,  $Q_s = \frac{\gamma a_{is} z_{is}}{w_{is}\sigma_{is}^2} - \frac{\gamma^2}{2} \frac{a_{is}^2}{\sigma_{is}^2 w_{is}^2}$ , we  
 715 have  $\gamma B_{it} - \frac{\gamma^2}{2} A_{it}^2 = \sum_{s=1}^{t-1} Q_s$ . Let  $\mathcal{F}_t = \sigma(\{A_{is}, X_{is}\}_{s=1}^{t-1})$  denote the  $\sigma$ -field generated by  
 716 observations reported by all users. Then  $\{\mathcal{F}_t\}_{t \geq 0}$  is a filtration and moreover  $a_{it}$  is  $\mathcal{F}_t$  measurable.  
 717 Therefore, by the sub-Gaussian condition (14),

$$\mathbb{E}[e^{Q_s} | \mathcal{F}_s] = \exp\left(-\frac{\gamma^2}{2} \frac{a_{is}^2}{\sigma_{is}^2 w_{is}^2}\right) \mathbb{E}\left[\exp\left(-\frac{\gamma a_{is}}{\sigma_{is}^2 w_{is}} z_{is}\right) \middle| \mathcal{F}_s\right] \leq 1.$$

718 Therefore,

$$\mathbb{E}\left[e^{\sum_{s=1}^{t-1} Q_s}\right] = \mathbb{E}\left[e^{\sum_{s=1}^{t-2} Q_s} \mathbb{E}[e^{Q_{t-1}} | \mathcal{F}_{t-1}]\right] \leq \mathbb{E}\left[e^{\sum_{s=1}^{t-2} Q_s}\right] \leq \dots \leq 1.$$

719 By applying Lemma 11 with a given  $\delta' \in (0, 1/e)$ , the following is true with probability greater than  
 720  $1 - \delta'$ .

$$|B_{it}| \leq A_{it} \sqrt{(4 + 2 \log(2)) \log(1/\delta')}. \quad (15)$$

721 **Step 2:** In this part of the proof, we will bound the estimation error  $|\theta_{it} - \theta_i^*|$  (see (4)) for the  
 722 parameter  $\theta_i^*$  in terms of  $B_{it}$ . This part of the analysis is based on prior work on generalised linear  
 723 models [21]. We first define,

$$g_{it}(\theta) = \sum_{s=1}^{t-1} \frac{a_{is}}{w_{is}\sigma_{is}^2} \mu\left(\frac{a_{is}}{w_{is}} \theta\right).$$

724 By an application of the mean value theorem we have,

$$|\theta_{it} - \theta_i^*| \leq \frac{1}{\dot{g}_{it}(\theta'_{it})} |g_{it}(\theta_{it}) - g_{it}(\theta_i^*)| \leq \frac{1}{\kappa_{\dot{\mu}} A_{it}^2} |g_{it}(\theta_{it}) - g_{it}(\theta_i^*)|$$

725 Here  $\theta'_{it}$  is between  $\theta_{it}$  and  $\theta_i^*$ . We have upper bounded its integral using our assumptions in  
 726 Section 3.2 to obtain  $\dot{g}_{it}(\theta'_{it}) \sum_{s=1}^{t-1} \frac{a_{is}^2}{w_{is}^2 \sigma_{is}^2} \dot{\mu}\left(\frac{a_{is}}{w_{is}} \theta'_{it}\right) \geq \kappa_{\dot{\mu}} A_{it}^2$ .

727 Next, let  $\theta_{it}^{\text{ML}}$  be the unique  $\theta \in \mathbb{R}$  satisfying  $g_{it}(\theta) = \sum_{s=1}^{t-1} \frac{a_{is}}{w_{is}\sigma_{is}^2} X_{is}$ . Readers familiar with  
 728 the literature on generalised linear models will recognise  $\theta_{it}^{\text{ML}}$  as the quasi-maximum likelihood  
 729 estimator [21]. We can therefore rewrite  $\theta_{it}$  in (4) as  $\theta_{it} = \operatorname{argmin}_{\theta > \theta_{\min}} |g_{it}(\theta) - g_{it}(\theta_{it}^{\text{ML}})|$ . We  
 730 therefore have,

$$\begin{aligned} |\theta_{it} - \theta_i^*| &\leq \frac{1}{\kappa_{\dot{\mu}} A_{it}^2} |g_{it}(\theta_{it}) - g_{it}(\theta_i^*)| \leq \frac{1}{\kappa_{\dot{\mu}} A_{it}^2} (|g_{it}(\theta_{it}) - g_{it}(\theta_{it}^{\text{ML}})| + |g_{it}(\theta_{it}^{\text{ML}}) - g_{it}(\theta_i^*)|) \\ &\leq \frac{2}{\kappa_{\dot{\mu}} A_{it}^2} |g_{it}(\theta_{it}^{\text{ML}}) - g_{it}(\theta_i^*)| = \frac{2}{\kappa_{\dot{\mu}} A_{it}^2} |B_{it}|. \end{aligned} \quad (16)$$

731 The last step follows from the definition of  $\theta_{it}$ .

732 **Step 3:** We now apply (15) with  $\delta' \leftarrow 6\delta/(\pi^2 n |D_t|^2)$  which is less than  $1/e$  if  $n \geq 2$ . By (16), a  
 733 union bound, and observing  $\sum t^{-2} = \pi^2/6$ , we have, with probability greater than  $1 - \delta$ ,

$$\text{for all } i, t, \quad |\theta_{it} - \theta_i^*| \leq \frac{2}{\kappa_{\dot{\mu}} A_{it}^2} \sqrt{4 + 2 \log(2)} A_{it} \leq \frac{\beta_t}{A_{it}}.$$

734 This establishes the result for the confidence intervals for  $\theta_i^*$ . The result for the confidence intervals  
 735 for  $\eta_i^*$  follows from the fact that  $\eta_i^* = \mu^{-1}(\alpha)/\theta_i^*$  is a decreasing function of  $\theta_i^*$ .  $\square$



## 736 D.2 Proof of Theorem 3

737 We will first state a complete version of Theorem 3 below. We will begin by defining a few quantities.  
738 First, let  $\gamma_t$  be as defined below.

$$\gamma_t = \beta_t \kappa_{\dot{\mu}} = 5\sqrt{\log(n\pi^2|D_t|^2/6\delta)}. \quad (17)$$

739 Additionally, define the following constant,

$$C = \frac{\sqrt{2}(\max_i \eta_i) w_{\max}^2 \sigma_{\max}}{\theta_{\min} \kappa_{\dot{\mu}} (\min_i e_i)}. \quad (18)$$

740 **Theorem** (Theorem 3 in full). *The following statements are true with probability greater than  $1 - \delta$*   
741 *for Algorithm 2 under the assumptions in Section 3.2. It is strategy-proof. It is fair, i.e.,  $U_{iT}^{e_i} \leq U_{iT}$*   
742 *for all  $i \in \{1, \dots, n\}$ . Under truthful reporting from all agents, it is asymptotically efficient with,*

$$L_T \leq 3T^{2/3} + 3Cn\gamma_T T^{2/3} \in \mathcal{O}\left(nT^{2/3}\sqrt{\log(nT/\delta)}\right), \quad \text{for all } T > 0.$$

743 *Proof.* Throughout this proof we will assume that for all  $i, n$ ,  $d_{it}^* \in (\tilde{d}_{it}, \hat{d}_{it})$ . By Lemma 13, this is  
744 true with probability at least  $1 - \delta$ .

745 **Efficiency:** This proof will follow a similar template to the proof for efficiency for the deterministic  
746 model. We will first decompose the loss as follows,

$$L_T \leq \sum_{t \in \mathbf{E}} \ell_t + \sum_{t \notin \mathbf{E}} \ell_t \leq q_T + \sum_{t \notin \mathbf{E}} \ell_t \leq 3T^{2/3} + \sum_{t \notin \mathbf{E}} \sum_{i=1}^n (\hat{d}_{it} - \tilde{d}_{it}).$$

747 We have used the fact that in  $T$  rounds there will have been  $q_T$  exploration rounds and then used  
748 Lemma 10 to upper bound  $q_T$ . To bound the second sum, we have used Lemma 6. Here,  $\hat{d}_{it} = w_{it}\hat{\eta}_{it}$   
749 and  $\tilde{d}_{it} = w_{it}\tilde{\eta}_{it}$  are upper and lower confidence bounds on the instantaneous demands, where  $\hat{\eta}_{it}, \tilde{\eta}_{it}$   
750 are the upper and lower confidence bounds on the unit demand as given in (5). We can bound this  
751 further via,

$$(\hat{d}_{it} - \tilde{d}_{it}) = \frac{\mu^{-1}(\alpha_i)w_{it}}{\tilde{\theta}_{it}\hat{\theta}_{it}} (\tilde{\theta}_{it} - \hat{\theta}_{it}) \leq \frac{2\eta_i^* w_{\max}}{\theta_{\min}} \frac{\beta_t}{A_{it}} \leq 2C\gamma_t t^{-1/3}$$

752 Here, the last step upper bounds  $A_{it}$  as follows; for this, we use Lemma 10 and the fact that at all  
753 exploration rounds agent  $i$  receives an allocation  $e_i$ .

$$A_{it}^2 = \sum_{s \in D_t} \frac{a_{is}^2}{w_{is}^2 \sigma_{is}^2} \geq \frac{e_i^2}{w_{\max}^2 \sigma_{\max}^2} q_t \geq \frac{e_i^2}{2w_{\max}^2 \sigma_{\max}^2} t^{2/3}.$$

754 This leads us the following bound on  $L_T$ ,

$$L_T \leq 3T^{2/3} + 2C\gamma_T \sum_{i=1}^n \sum_{t \notin \mathbf{E}} t^{-1/3} \leq 3T^{2/3} + 3Cn\gamma_T T^{2/3}.$$

755 **Fairness:** This follows as a direct consequence of Lemma 7. During the exploration phase rounds,  
756 each agent gets her entitlement  $a_{it} = e_i$ . During the other rounds, we invoke MMF using an upper  
757 bound on the agent's demand, and therefore the RHS of Lemma 7 is 0 for these rounds.

758 **Strategy-proofness:** This follows from Lemma 8 as we use  $\hat{\eta}_i \leftarrow \hat{\eta}_{it}$  which is an upper bound on  $\eta_i^*$   
759 when the confidence intervals trap the true parameter.  $\square$

## 760 D.3 Proof of Theorem 4

761 We will first state a complete version of Theorem 4 below. For this, define the following constants.

$$C_1 = \frac{\theta_{\min} \kappa_{\dot{\mu}}}{2\sigma_{\max} w_{\max}}, \quad C_2 = \frac{1}{\sqrt{\log(1 + C_1^2)}}, \quad C_3 = \frac{\sigma_{\max} w_{\max}}{\sigma_{\min} w_{\min} \min_i e_i^2}. \quad (19)$$

762 We now state the theorem.



**Theorem** (Theorem 4 in full). Let  $\gamma_T$  be as defined in (17) and  $C_2, C_3$  be as defined in (19). The following statements are true with probability greater than  $1 - \delta$  for Algorithm 3 under the assumptions in Section 3.2. It is fair, i.e.,  $U_{iT}^{e_i} \leq U_{iT}$  for all  $i \in [n]$ . Under truthful reporting from all agents, it is asymptotically efficient with,

$$L_T \leq 1 + C_2 n \gamma_T T^{1/2} \sqrt{\log(C_3 T)} \in \mathcal{O}\left(n T^{1/2} \sqrt{\log(nT/\delta) \log(T)}\right),$$

for all  $T \geq 0$ . Finally, assume all agents except  $i$  are truthful. Let  $U_{iT}, U_{iT}^\pi$  respectively denote the sum of utilities when  $i$  participates truthfully and when she is following any other (non-truthful) policy  $\pi$ . Then, for all  $\pi$ , for all  $T > 0$ ,

$$U_{iT}^\pi - U_{iT} \leq \frac{L_i C_2}{w_{\min}} (n-1) \gamma_T \sqrt{(T-1) \log(C_3 T)} \in \mathcal{O}\left(n T^{1/2} \sqrt{\log(nT/\delta) \log(T)}\right).$$

We will begin with three intermediate lemmas. The first will help us establish the result for asymptotic efficiency, the second will help us with asymptotic fairness, and the third is a technical lemma that will help us in controlling both loss terms. In all three lemmas, we will let  $\mathcal{E}$  denote the event that for all  $i, n$   $d_{it}^* \in (\tilde{d}_{it}, \hat{d}_{it})$ . By Lemma 13,  $\mathbb{P}(\mathcal{E}) \geq 1 - \delta$ .

**Lemma 14.** The following bound holds on  $L_T$  under event  $\mathcal{E}$ .

$$L_T \leq 1 + \frac{\gamma_T}{C_1} \sum_{i=1}^n \sum_{t=2}^T \min\left(C_1, \frac{a_{it}}{w_{it} \sigma_{it} A_{it}}\right).$$

*Proof.* We will divide this proof into three steps. In the first two steps, we will consider a single round  $t \geq 2$ . Recall the notation at the beginning of Appendix B.

**Step 1:** First, we will argue that  $\ell_t \leq \min(1, \ell_t^{\text{or}})$ . Observe that if  $\ell_t^{\text{ur}} = 0$ , then  $a_t = \hat{d}_{it} \geq d_{it}^*$  and therefore  $\ell_t \leq \ell_t^{\text{ud}} = 0$  and the claim is true. When  $\ell_t^{\text{ur}} = 0$ , then we can bound  $\ell_t \leq \ell_t^{\text{ur}} + \ell_t^{\text{or}} = \ell_t^{\text{or}}$ . The above claim follows by observing that  $\ell_t \leq 1$  trivially since the total amount of the resource is 1.

**Step 2:** Next, consider any user  $i$ . We will argue that  $\max(a_{it} - d_{it}^*, 0) \leq \frac{2\beta_t}{\theta_{\min}} \frac{a_{it}}{A_{it}}$ . Let  $\{a_{jt}^*\}_{j=1}^n$  denote the allocations returned by MMF if we were to invoke with the true demands  $\{d_{jt}^*\}_{j=1}^n$  for round  $t$ . Recall that  $a_{it}^* \leq d_{it}^*$ .

First assume  $a_{it}^* < d_{it}^*$ . Then, by Property 3, increasing  $i$ 's reported demand to  $\hat{d}_{it} (> d_{it}^*)$  while keeping the demands of all other agents at  $\{d_{jt}^*\}_{j \neq i}$  does not increase  $i$ 's allocation. Moreover, increasing the demands of all other agents cannot increase  $i$ 's allocation and hence  $a_{it} \leq a_{it}^* < d_{it}^*$ ; therefore, the statement is true since the RHS is positive.

Now assume  $a_{it}^* = d_{it}^*$ . If  $a_{it} \leq a_{it}^* = d_{it}^*$ , the statement is trivially true. Therefore, let  $a_{it} > a_{it}^* = d_{it}^* > \tilde{d}_{it}$ . As MMF does not allocate more than the reported demand, we also have  $a_{it} < \hat{d}_{it}$ . This results in the following bound.

$$\max(a_{it} - d_{it}^*, 0) \leq \hat{d}_{it} - \tilde{d}_{it} \leq \frac{\mu^{-1}(\alpha)}{\tilde{\theta}_{it} \hat{\theta}_{it}} (\hat{\theta}_{it} - \tilde{\theta}_{it}) \leq \frac{\tilde{d}_{it}}{\tilde{\theta}_{it}} \frac{2\beta_t}{A_{it}} \leq \frac{2\beta_t}{\theta_{\min}} \frac{a_{it}}{A_{it}}.$$

**Step 3:** We now combine the results of the previous two steps to bound  $L_T$  as follows.

$$\begin{aligned} L_T &= \sum_{t=1}^T \ell_t \leq 1 + \sum_{t=2}^T \ell_t \leq 1 + \sum_{t=2}^T \min(1, \ell_t^{\text{ur}}) = 1 + \sum_{t=2}^T \min\left(1, \sum_{i=1}^n \max(a_{it} - d_{it}^*, 0)\right) \\ &\leq 1 + \sum_{t=2}^T \sum_{i=1}^n \min(1, \max(a_{it} - d_{it}^*, 0)) \leq 1 + \sum_{t=2}^T \sum_{i=1}^n \min\left(1, \frac{2\beta_t}{\theta_{\min}} \frac{a_{it}}{A_{it}}\right) \\ &\leq 1 + \sum_{i=1}^n \sum_{t=2}^T \min\left(1, \frac{2\gamma_t \sigma_{it} w_{it}}{\kappa_{\mu} \theta_{\min}} \frac{a_{it}}{\sigma_{it} w_{it} A_{it}}\right) \leq 1 + \gamma_T \sum_{i=1}^n \sum_{t=2}^T \min\left(1, \frac{1}{C_1} \frac{a_{it}}{\sigma_{it} w_{it} A_{it}}\right) \\ &\leq 1 + \frac{\gamma_T}{C_1} \sum_{i=1}^n \sum_{t=2}^T \min\left(C_1, \frac{a_{it}}{\sigma_{it} w_{it} A_{it}}\right) \end{aligned} \tag{20}$$

Here, the third step applies the results from step 1. The fifth step simply uses  $\min(a, \sum_i b_i) \leq \sum_i \min(a, b_i)$  when  $b_i \geq 0$  for all  $i$ . The sixth step applies the result from step 2. The eighth step uses the fact that  $\gamma_t \geq 1$ .  $\square$

**Lemma 15.** Consider any agent  $i \in \{1, \dots, n\}$  and assume all other agents are submitting truthfully. Let  $U_{iT}^\pi, U_{iT}$  be as defined in Theorem 4. The following bound holds on  $U_{iT}^\pi - U_{iT}$  under event  $\mathcal{E}$ .

$$U_{iT}^\pi - U_{iT} \leq \frac{L_i \gamma_T}{C_1 w_{\min}} \sum_{j \neq i} \sum_{t=2}^T \min \left( C_1, \frac{a_{jt}}{w_{jt} \sigma_{jt} A_{jt}} \right).$$

796

*Proof.* We will divide this proof into three steps.

**Step 1:** We will decompose  $U_{iT}^\pi - U_{iT}$  as follows. Let  $u_{it}^\pi$  denote the utility at time  $t$  when agent  $i$  is following  $\pi$ . Let  $u_{it}^\dagger$  denote the utility at time  $t$  when agent  $i$  follows  $\pi$  until round  $t-1$  and then on round  $t$  we invoke MMF (line 5, Algorithm 3) with the true demand  $d_{it}^* = \eta_i^* w_{it}$  for agent  $i$ , and the upper bounds  $\hat{d}_{jt} = \hat{\eta}_{jt} w_{jt}$  for all other agents  $j$ . Let  $u_{it}^*$  denote the utility of agent  $i$  when we invoke MMF with the true demands for all agents. We then have,

$$U_{iT}^\pi - U_{iT} = \sum_{t=1}^n (u_{it}^\pi - u_{it}) = \sum_{t=1}^n (u_{it}^\pi - u_{it}^\dagger + u_{it}^\dagger - u_{it}^* + u_{it}^* - u_{it}) = \sum_{t=1}^n (u_{it}^* - u_{it}).$$

The last step is obtained via two observations. First,  $u_{it}^\pi - u_{it}^\dagger \leq 0$  since, by Theorem 5, reporting true demands is a weakly dominant strategy for agent  $i$ . Second,  $u_{it}^\dagger - u_{it}^* \leq 0$  since the reported demands used for all other agents  $j \neq i$  is an upper bound on their true demands under  $\mathcal{E}$  as they are being truthful; in the reported demands for MMF in  $u_{it}^\dagger, u_{it}^*$ , agent  $i$ 's reported demand stays the same but the reported demands of other agents decrease, which cannot decrease the allocation of agent  $i$ .

Next, using the Lipschitz properties of  $u_i$ , we can write  $u_{it}^* - u_{it} = u_i(a_{it}^*/w_{it}) - u_i(a_{it}/w_{it}) \leq L_i \max(a_{it}^*/w_{it} - a_{it}/w_{it}, 0) \leq \frac{L_i}{w_{\min}} \max(a_{it}^* - a_{it}, 0)$ . Moreover, since increasing all user's demands can only increase the sum of allocations, we have  $\sum_{j=1}^n a_{jt}^* \leq \sum_{j=1}^n a_{jt}$ . Therefore,  $a_{it}^* - a_{it} \leq \sum_{j \neq i} (a_{jt} - a_{jt}^*)$  and hence  $\max(a_{it}^* - a_{it}, 0) \leq \sum_{j \neq i} \max(a_{jt} - a_{jt}^*, 0)$ . This leads us to the following bound.

$$U_{iT}^\pi - U_{iT} \leq \frac{L_i}{w_{\min}} \sum_{t=1}^n \max(a_{it}^* - a_{it}, 0) \leq \frac{L_i}{w_{\min}} \sum_{t=1}^n \sum_{j \neq i} \max(a_{jt} - a_{jt}^*, 0).$$

**Step 2:** Consider any user  $j \neq i$ . Here, we will argue that  $\max(a_{jt} - a_{jt}^*, 0) \leq \frac{2\beta_t}{\theta_{\min}} \frac{a_{jt}}{A_{jt}}$ , where, recall  $\{a_{kt}^*\}_{k=1}^n$  is the allocation returned by MMF if we use the true demands  $\{d_{kt}^*\}_{k=1}^n$  for all agents  $k$ . First observe that if  $a_{jt} \leq a_{jt}^*$ , the statement is trivially true as the RHS is positive.

Next, if  $a_{jt} > a_{jt}^*$ , we argue that  $a_{jt}^* = d_{jt}^*$ ; we will prove this via its contrapositive. Observe that  $a_{jt}^* \leq d_{jt}^*$  by properties of MMF. Let us assume that  $a_{jt}^* < d_{jt}^*$ . Then, by Property 3, increasing  $j$ 's reported demand to  $\hat{d}_{jt} (> d_{jt}^*)$  while keeping the reported demands of all other agents at  $\{d_{kt}^*\}_{k \neq j}$  does not increase her allocation. Next, increasing the demands of all other agents cannot increase  $j$ 's allocation and hence  $a_{jt} \leq a_{jt}^*$ . This proves the above statement. By substituting  $d_{jt}^*$  for  $a_{jt}^*$ , we obtain the following bound.

$$\max(a_{jt} - a_{jt}^*, 0) \leq \hat{d}_{jt} - \check{d}_{jt} \leq \frac{\mu^{-1}(\alpha)}{\check{\theta}_{jt} \hat{\theta}_{jt}} (\hat{\theta}_{jt} - \check{\theta}_{jt}) \leq \frac{\check{d}_{jt}}{\check{\theta}_{jt}} \frac{2\beta_t}{A_{jt}} \leq \frac{2\beta_t}{\theta_{\min}} \frac{a_{jt}}{A_{jt}}.$$

Above, we have used the facts  $a_{jt} \leq \hat{d}_{jt}$ ,  $d_{jt}^* \geq \check{d}_{jt}$ , and the expressions for  $\hat{d}_{jt}, \check{d}_{jt}, \hat{\theta}_{jt}, \check{\theta}_{jt}$ .

**Step 3:** Combining the results of the two previous steps, we obtain the following bound,

$$U_{iT}^\pi - U_{iT} \leq \frac{L_i}{w_{\min}} \sum_{t=1}^n \sum_{j \neq i} \min \left( 1, \frac{2\beta_t}{\theta_{\min}} \frac{a_{jt}}{A_{jt}} \right) \leq \frac{L_i \gamma_T}{C_1 w_{\min}} \sum_{j \neq i} \sum_{t=2}^T \min \left( C_1, \frac{a_{jt}}{w_{jt} \sigma_{jt} A_{jt}} \right).$$

Here, the first step observes that  $\max(a_{jt} - a_{jt}^*, 0) \leq 1$  and the last step is obtained by repeating the calculations in (20).  $\square$

826 **Lemma 16.** Let  $c > 0$ . Then,  $\sum_{t=1}^T \min \left( c, \frac{a_{it}^2}{\sigma_{it}^2 w_{it}^2 A_{it}^2} \right) \leq \frac{c}{\log(1+c)} \log(C_3 T)$ .

827 *Proof.* We first simplify  $A_{iT}^2$  as follows.

$$A_{iT}^2 = A_{i,T-1}^2 + \frac{a_{iT}^2}{w_{iT}^2 \sigma_{iT}^2} = A_{i,T-1}^2 \left( 1 + \frac{a_{iT}^2}{A_{i,T-1}^2 w_{iT}^2 \sigma_{iT}^2} \right) = \dots = A_{i2}^2 \prod_{s=1}^{T-1} \left( 1 + \frac{a_{is}^2}{A_{is}^2 w_{is}^2 \sigma_{is}^2} \right)$$

828 Now, observing that  $A_{iT}^2 = \sum_{t=1}^{T-1} \frac{a_{it}^2}{\sigma_{it}^2 w_{it}^2} \leq \frac{T-1}{\sigma_{\min} w_{\max}}$  and that  $A_{i2}^2 = \frac{e_i^2}{\sigma_{i1}^2 w_{i1}} \geq \frac{e_i^2}{\sigma_{\max} w_{\max}}$ , we obtain,

$$\sum_{t=1}^T \log \left( 1 + \frac{a_{it}^2}{\sigma_{it}^2 w_{it}^2 A_{it}^2} \right) = \log \left( \frac{A_{iT}^2}{A_{i2}^2} \right) \leq \log(C_3 T).$$

829 By applying Lemma 12, we obtain

$$\sum_{t=1}^T \min \left( c, \frac{a_{it}^2}{\sigma_{it}^2 w_{it}^2 A_{it}^2} \right) \leq \frac{c}{\log(1+c)} \sum_{t=1}^T \log \left( 1 + \frac{a_{it}^2}{\sigma_{it}^2 w_{it}^2 A_{it}^2} \right) \leq \frac{c}{\log(1+c)} \log(C_3 T).$$

830 □

831 We are now ready to prove the theorem.

832 *Proof of Theorem 4.* In this proof, denote  $Q_i = \sum_{t=2}^T \min \left( C_1, \frac{a_{it}}{w_{it} \sigma_{it} A_{it}} \right)$ . By an application of  
833 the Cauchy-Schwarz inequality and Lemma 16 we obtain,

$$Q_i^2 \leq (T-1) \sum_{t=2}^T \min \left( C_1^2, \frac{a_{it}^2}{w_{it}^2 \sigma_{it}^2 A_{it}^2} \right) \leq (T-1) C_1^2 C_2^2 \log(C_3 T).$$

834 **Efficiency:** The claim for asymptotic efficiency follows by applying Lemma 14.

$$L_T \leq 1 + \frac{\gamma_T}{C_1} \sum_{i=1}^n Q_i \leq 1 + C_2 n \gamma_T \sqrt{(T-1) \log(C_3 T)}.$$

835 **Fairness:** Similar to the argument in Appendix D.2, this follows as a direct consequence of Lemma 7.  
836 On round 1, each agent gets her entitlement. On each subsequent round, we invoke MMF using an  
837 upper bound on the agent's demand.

838 **Strategy-proofness:** The claim for asymptotic Bayes-Nash incentive compatibility follows by  
839 applying Lemma 15.

$$U_{iT}^\pi - U_{iT} \leq \frac{L_i \gamma_T}{C_1 w_{\min}} \sum_{i=1}^n Q_i \leq \frac{L_i C_2}{w_{\min}} (n-1) \gamma_T \sqrt{(T-1) \log(C_3 T)}.$$

840 □

841 **Remark 2.** In our proofs, if  $\sigma_{it} = 0$ , then many of the above quantities become undefined. If at any  
842 instant  $\sigma_{it} = 0$ , it means we will have observed  $f_{\theta_i^*}$  at  $a_{it}/w_{it}$  exactly, and will know  $\theta_i^*$ . Since,  $f_{\theta_i^*}$   
843 is completely determined by  $\theta_i^*$ , we can compute the agent's true unit demand and use it from thereon.  
844 We also require  $w_{it} > 0$  for the strategy-proof case for a similar reason as in Remark 1 and can be  
845 avoided by a more careful analysis which only accounts for time indices where  $w_{it} > 0$ .

## 846 E Addendum to Experiments Section

847 We provide some details on the experimental set up.

## 848 Implementation Details

849 For the stochastic methods, we solved for  $\theta_{it}$  in (4), by first computing  $\theta_{it}^{\text{ML}}$  as given in Appendix D,  
850 and then clipping it at  $\theta_{\min}$ . However, in practice we found  $\theta_{it}^{\text{ML}} > \theta_{\min}$  in almost all cases. We  
851 solved for  $\theta_{it}^{\text{ML}}$ , using the Newton-Raphson method.

852 In all our experiments, we used  $\delta = 10^{-3}$ . We found the theoretical value for  $\beta_t$  as given in  
853 Section 3.2 to be too conservative; therefore, we divided it by 10. This value was tuned using a  
854 hold-out set of synthetic experiments that were not included in Figure 1. Note that it is common to  
855 tune upper confidence bounds in a similar manner in the bandit literature [21].

## 856 The Prediction Serving Task

857 We evaluate our approach on latency-sensitive prediction serving [16], which is used in applications  
858 such as alarm systems [50] and Amazon Alexa [1]. In this setting, the user deploys a queued serving  
859 system that takes query inputs and returns prediction responses. Due to the real-time nature of these  
860 applications, sub-second response time is expected. This setting is of particular interest because  
861 although the application owner knows how to quantify strict performance requirements from the  
862 application, the appropriate resource allocation is far less clear a priori, due to the complexity of the  
863 system.

864 In our experiment we consider 5 such users, with equal entitlement to 100 VMs. Each user specifies  
865 a 100ms, 0.99 percentile latency SLO target for their application response time, meaning that they  
866 allow at most 1% of queries in incoming traffic to have response time greater than 100ms. At the end  
867 of each round, users provide feedback on the fraction of queries that were completed on time. For the  
868 arrival traffic of 3 of the users we use varying time-of-day and day-of-week regions in the Waikato  
869 network dataset [37], for one of them we use data from the Twitter streaming API [7], and for one we  
870 use the Wikipedia traffic data [8]. We use a query-level execution simulator from [16], which uses  
871 power-of-2-choices load balancing to mimic real deployment conditions.
